# Supplementary material for: Community Detection in Directed Weighted Networks using Voronoi Partitioning
Source: arXiv:2304.12389 source file (2023-04-24)
Supplement: Supplementary file 1 [file Supplementary_Information.pdf]

Supplementary Information for

# Community Detection in Directed Weighted Networks using Voronoi Partitioning

Molnár et al.

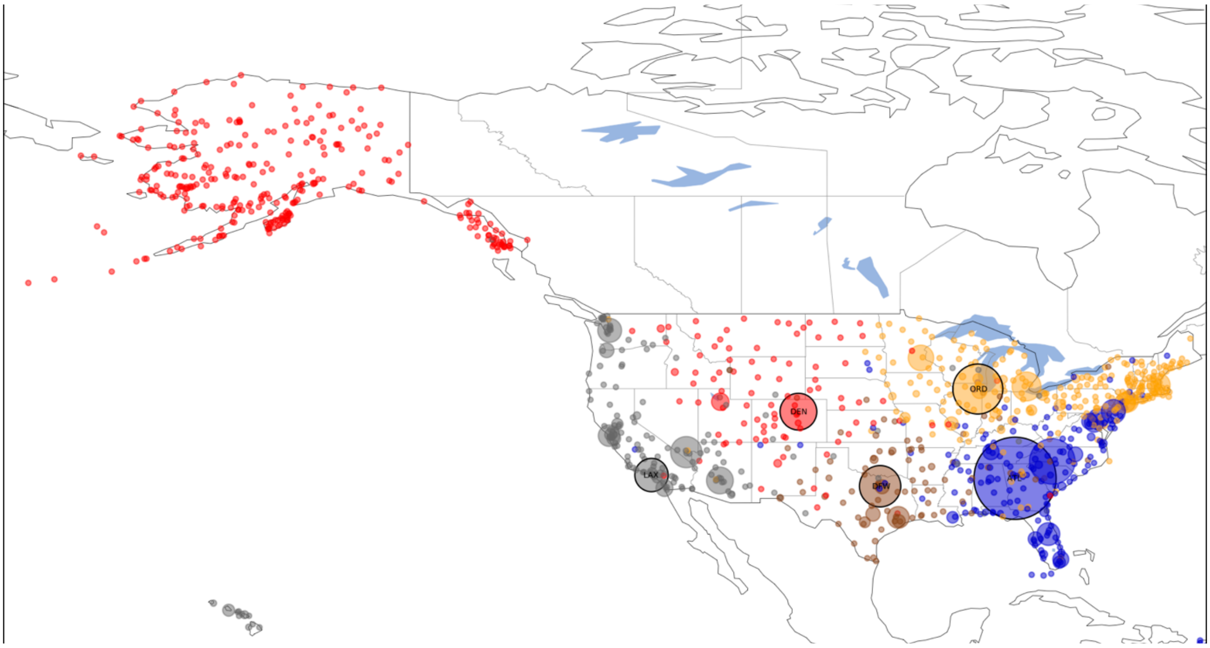


**Supplementary Figure 1.** Clustering of the air passenger transportation network of the United States using the Voronoi algorithm using the Top 5 busiest airports (ATL, LAX, ORD, DFW, DEN) as generator points. The dots represent the locations of airports on the map, their size is proportional to the local density. Colors represent the different clusters; the black border indicates the generator nodes. Only generator point airports display the IATA airport code.

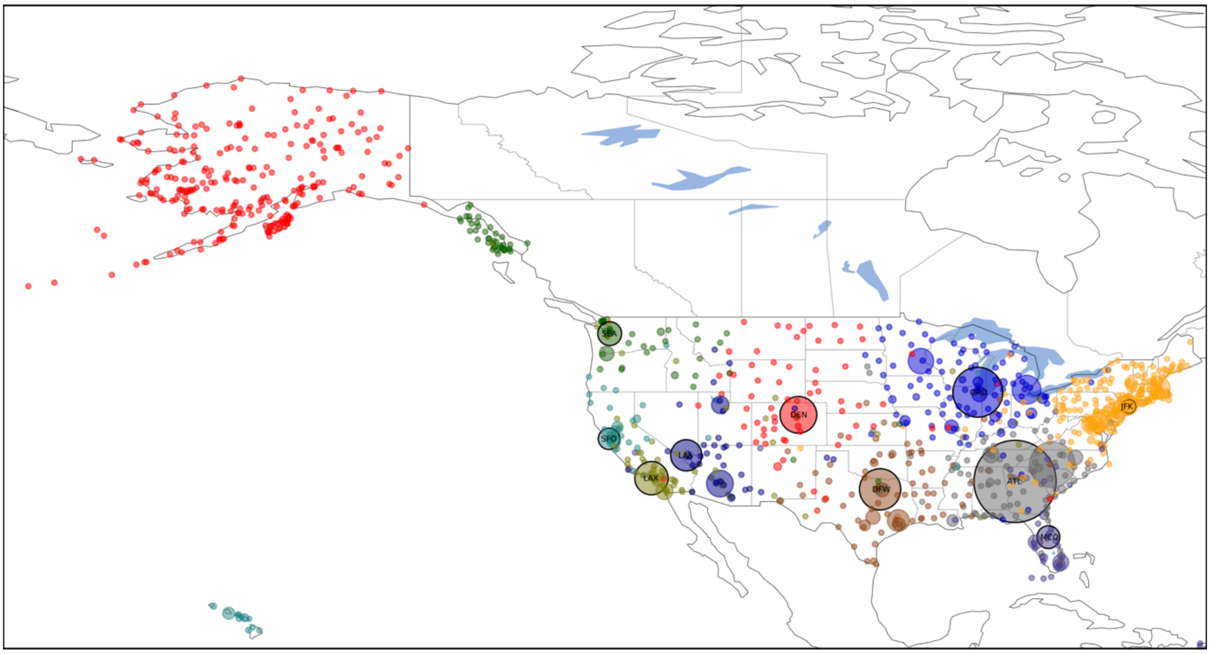


**Supplementary Figure 2.** Clustering of the air passenger transportation network of the United States using the Voronoi algorithm using the Top 10 busiest airports (ATL, LAX, ORD, DFW, DEN, JFK, SFO, SEA, LAS, MCO) as generator points. The dots represent the locations of airports on the map, their size is proportional to the local density. Colors represent the different clusters; the black border indicates the generator nodes. Only generator point airports display the IATA airport code.

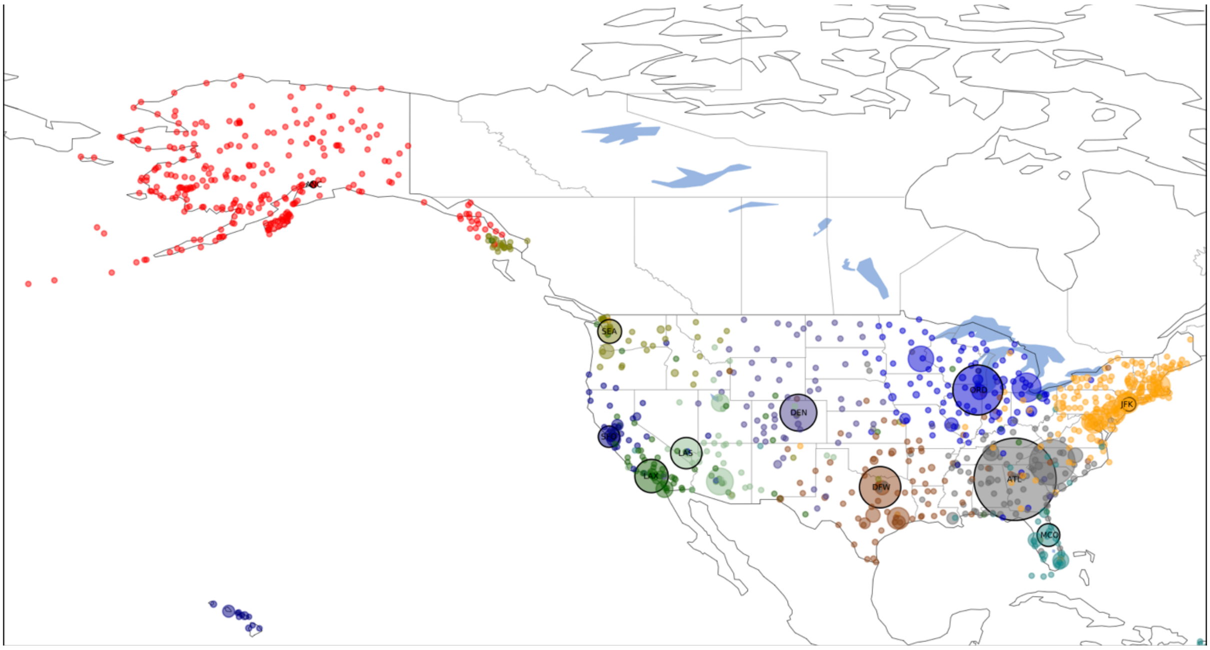


**Supplementary Figure 3.** Clustering of the air passenger transportation network of the United States using the Voronoi algorithm using the Top 10 busiest airports (ATL, LAX, ORD, DFW, DEN, JFK, SFO, SEA, LAS, MCO) and ANC as generator points. The dots represent the locations of airports on the map, their size is proportional to the local density. Colors represent the different clusters; the black border indicates the generator nodes. Only generator point airports display the IATA airport code.
